# Supplementary material for: Integrating planar circuits with superconducting 3D microwave cavities using tunable low-loss couplers
Source: arXiv:2304.06162 ancillary file (2023-06-15)
Supplement: Supplementary file 1 [file supp_6_12_23.pdf]

# Supplementary material for integrating planar circuits with superconducting 3D microwave cavities using tunable low-loss couplers

(Dated: 13 June 2023)

## A. Equipment photo and full experiment setup

Figure S1 shows a picture of the assembled device, with the chip, the coaxial quarter wave cavity and the a printed circuit board (PCB), which provides the interface between cryostat cabling and chip wiring for both the control lines and the microwave output. A copper lid (not shown in the figure) is used to cover the PCB board and chip. The slit where the chip mates with the cavity is 4 mm wide and 0.6 mm tall, machined by wire electrical discharge machining, which can achieve a tight tolerance of 10 $\mu$m. The dimensions are chosen to closely fit the width of the chip, while leaving an airgap above which minimizes the decay of the cavity field through the split. The chip itself is held in place by a thin layer of rubber cement.

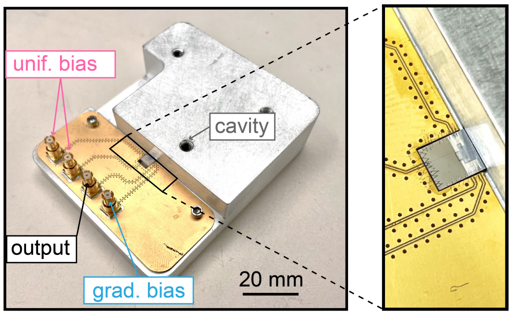


Fig. S1. The left device photo shows the aluminum body of the device, with the PCB, and partially inserted chip. The right image zooms in on the partially inserted chip.

We also show a full wiring diagram in Fig. S2. For the frequency domain data shown in the main text, we connect a VNA to the input and output ports at room temperature. For the time domain measurement, we use an IQ mixer to mix down the outgoing field from the output port from the cavity frequency to about 10 MHz, and digitize it with an analog-to-digital converter. In figure 2b of the main text, the amplitude of these complex signals are shown. The $E_{\text{stored}}$ in the main text are estimated from the microwave power injected into the cryostat and the attenuation of the lines, known to an accuracy of 1 dB.

## B. Coupling scheme in the terms of on-chip modes

We model our system as coupled modes and predict coupling rates, loss rates, and reflection amplitude from this model. We first identify the uncoupled modes in the system, and then engineer their resonance frequencies and the coupling rates between them, to optimize for the on/off ratio. In the uncoupled basis, where the loop is not inserted into the

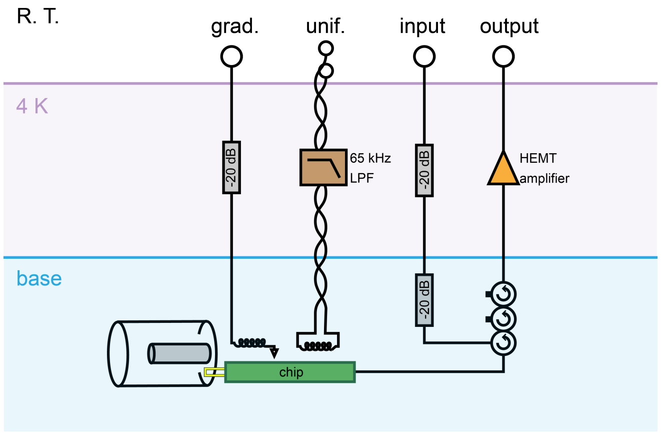


Fig. S2. Full wiring diagram of the experiment.

cavity and the bias is not applied, our model contains one cavity mode, and two chip modes on the TIB. For these two chip modes, one is coupled to the cavity (y-mode) when the loop antenna is inserted into the cavity, and the other (x-mode) is connected to the output port ( Fig. S3). The y-mode in turn has a variable coupling to the x-mode which is controlled by the TIB bias. One insight from this model is that the resonance of the y-mode needs to be detuned from that of the cavity to isolate the high quality factor of the cavity from loss on the chip. Series capacitors inserted in the connection between the TIB and the antenna both allow the y-mode resonance frequency to be adjusted and break an undesired superconducting loop.

## C. Loop antenna design

The loop antenna is a 10 um wide Nb trace arranged into a 3.5 mm by 1.0 mm rectangle, with the bottom edge cut in the middle and connected to a conductor-backed coplanar strip transmission line, serving as the antenna's feedline (Fig. S4a). When the antenna is not inserted into the cavity, it has an inductance of 9 nH, and is represented by a (yellow) inductor in Fig. 1b of the main text, and in Fig. S4b. When this loop is inserted into a cavity, the magnetic coupling coefficient is $k = 0.067$ (Fig. S4b).

The feedline, required to connected the TIB to the antenna, is a conductor-backed coplanar strip transmission line: 1636.5 $\mu$m long, 14 $\mu$m wide and with a 2 $\mu$m gap between the strips. This arrangement forms a 52 $\Omega$ transmission line with about 30 $^\circ$ electrical length at 6 GHz. The conductor back is connected to the cavity without seams because it is cut from same piece of metal as the cavity.

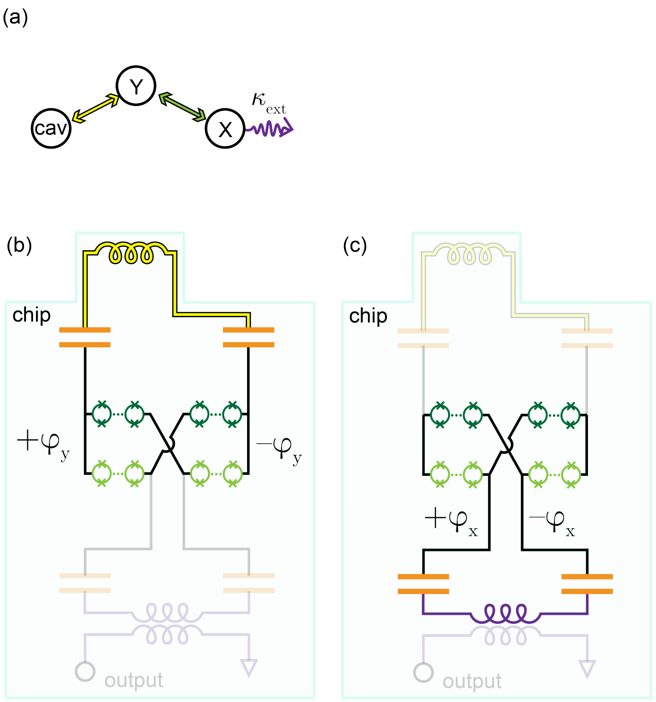


Fig. S3. Resonant modes in the system in the uncoupled case. a) The coupling between the cavity and the output port is mediated by 2 chip modes: x-mode and y-mode, defined below. The coupling between the cavity and the y-mode is shown as the yellow arrow, and the tunable coupling between the x-mode and y-mode is shown as the green arrow. b) The y mode frequency is determined by the bridge inductance, the loop inductance and the capacitors placed between them. This frequency is measured to be 8.4 GHz or 6.7 GHz when the coupler is turned off or on, respectively. c) The x mode frequency is determined by the bridge inductance, the balun inductance and the capacitors placed between them. This frequency is estimated from simulation to be 7.4 GHz or 6.7 GHz when the coupler is turned off or on, respectively.

## D. Establishing uniform current bias

The inductance of the SQUID arrays on opposing sides of the TIB is given by

$$L_{+/-} = \frac{NL_J}{2\left|\cos\left(\pi\frac{\Phi_u \pm \Phi_g}{\Phi_0}\right)\right|} \tag{S1}$$

Where $\Phi_0 = h/2e$ is the magnetic flux quantum, $L_J$ is the Josephson inductance, $N$ is the number of SQUIDs per array, $\Phi_u$ is the uniform flux, and $\Phi_g$ is the gradiometric flux. In our experiment, $L_J = 66$ pH and $N = 26$.

The uniform flux bias line threads the same flux through all the SQUID loops. By laying out the SQUID arrays in a gradiometric "figure-of-eight" arrangement, we prevent the uniform flux bias from penetrating the TIB bridge loop as shown in Fig S3. Without the uniform flux bias, the inductance is an even function of $\Phi_g$, such that inductances on adjacent arms of the TIB would not be different and we would not imbalance the bridge. From equation S1, we can see that to obtain the maximal imbalance of the bridge when we apply $\Phi_g$, $\Phi_u$ must be

$$\Phi_u = \Phi_0\left(\frac{1}{4} + \frac{n}{2}\right)$$

where $n$ is an integer.

To establish the uniform bias in the experiment, we set $\Phi_g$ close to zero and sweep the current in the uniform bias line, while monitoring the microwave reflection off of the TIB and cavity (Fig. S2). As expected, we observe that the cavity resonance is tuned periodically with the uniform bias because part of the cavity mode's energy is stored in the TIB's SQUID inductance. We find the current values at the maximum and minimum resonance frequencies and associate them with $\Phi_u = 0$ and $\Phi_u = \Phi_0/2$, respectively. We then set the uniform current bias to the average of these two values, corresponding to $\Phi_u = \Phi_0/4$. Then, we fix the current to that point and proceed with the experiment by tuning only $\Phi_g$ to imbalance the bridge (denoted as $\Phi$ in the main text).

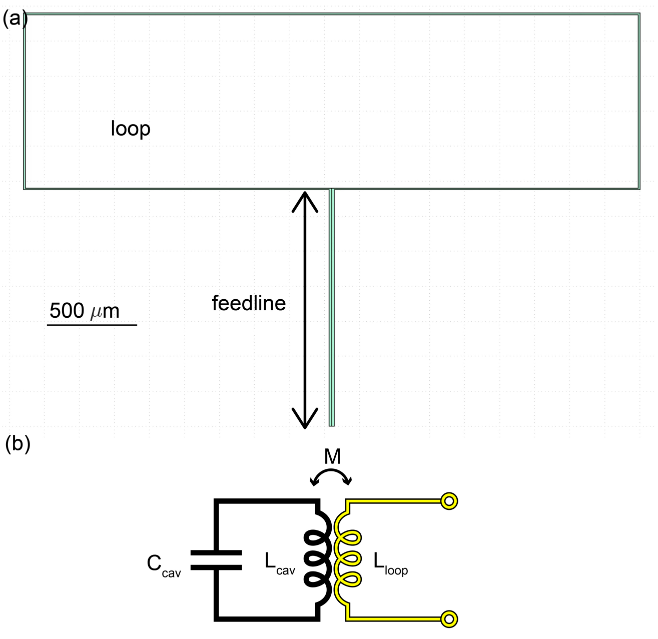


Fig. S4. Loop antenna design. a) The image shows the layout of the loop antenna and the feedline connecting to it. The bottom end of the feedline is then connected to the TIB via capacitors. b) A lumped-element transformer model describes the coupling between the cavity and the loop as a mutual inductance $M$, and with cavity itself modeled as an LC circuit with capacitance $C_{cav}$ and inductance $L_{cav}$. Finally, the loop antenna is modeled as an inductance $L_{loop}$. The dimensionless coupling of the transformer is $k = M/\sqrt{L_{cav}L_{loop}}$.

## E. Bounding the TIB OFF coupling

The ability of the TIB to either transmit a signal unaltered or (by inverting the gradiometric bias) to invert a signal is part

of the reason that it can have near zero transmission. Only a leakage component of a microwave signal that bypasses the TIB and is $\pi/2$ out of phase cannot be eliminated by adjusting the gradiometric bias. But in the experiments described in the main text, the sign inversion of the TIB is concealed because all microwave response measurements are performed in reflection and a signal that reflects from the cavity will have passed through the TIB twice. We therefore modified the wiring diagram shown in Fig. S2 to further bound the TIBs transmission in its OFF mode.

In a separate series of experiments, we added an additional weakly coupled port to the coaxial quarter wave cavity, and measured the transmission through the cavity and TIB as a function of gradiometric bias at the same uniform bias used in the main experiments. This result is shown in Fig. S5, where the prominent feature is the cavity resonance. As the bias is tuned, the phase of the transmitted signal clearly inverts where the transmission amplitude drops. The transmission at the phase inversion point is not resolved from zero, but it is at least 50 dB below its maximum value.

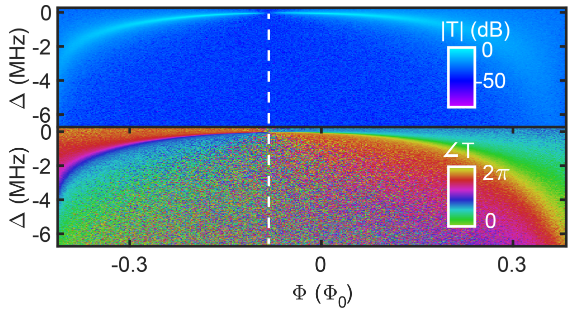


Fig. S5. Transmission (T) amplitude and phase is measured around cavity resonance frequency (Δ), when the bias is varied. The white dashed line indicates the OFF bias point.
